# Supplementary material for: Joint Monocular 3D Vehicle Detection and Tracking
Source: arXiv:1811.10742 source file (2019-09-12)
Supplement: Supplementary file 1 [file Truns.pdf]

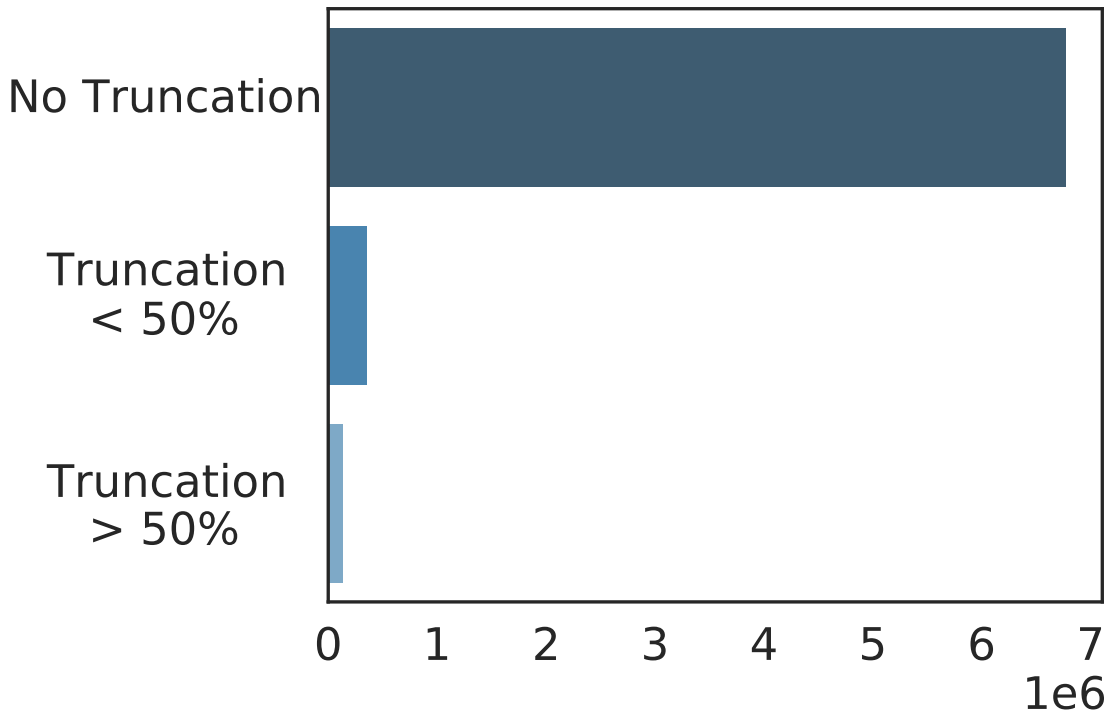

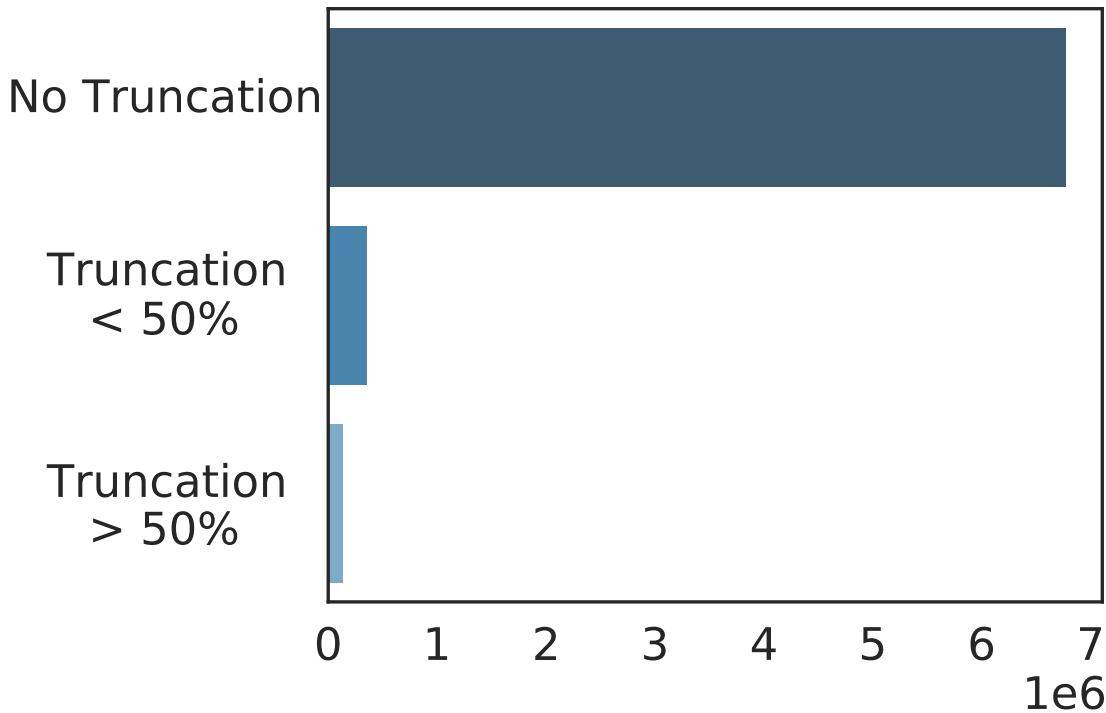

No Truncation

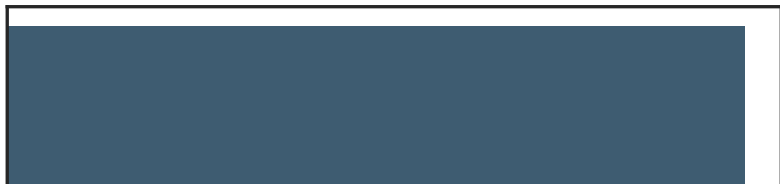

Truncation  
< 50%

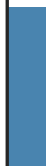

Truncation  
> 50%

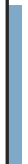

0 1 2 3 4 5 6 7  
1e6
